# Supplementary material for: A Survey on In-context Learning
Source: arXiv:2301.00234 source file (2024-10-05)
Supplement: Supplementary file 1 [file appendix.tex]

\section{Main Procedures of ICL}
The main procedures of ICL are illustrated in Fig.~\ref{fig:icl_process}. Pretraining is significant for developing the ICL ability of LLMs, and the optional warmup stage can further improve it. For the demonstrations, the most important procedure is demonstration design. With a pretrained LLM and a well-designed demonstration, a proper scoring strategy finally yield the task output.
% Directions current 
\begin{figure}[h]
    \centering
    \includegraphics[width=0.9\linewidth]{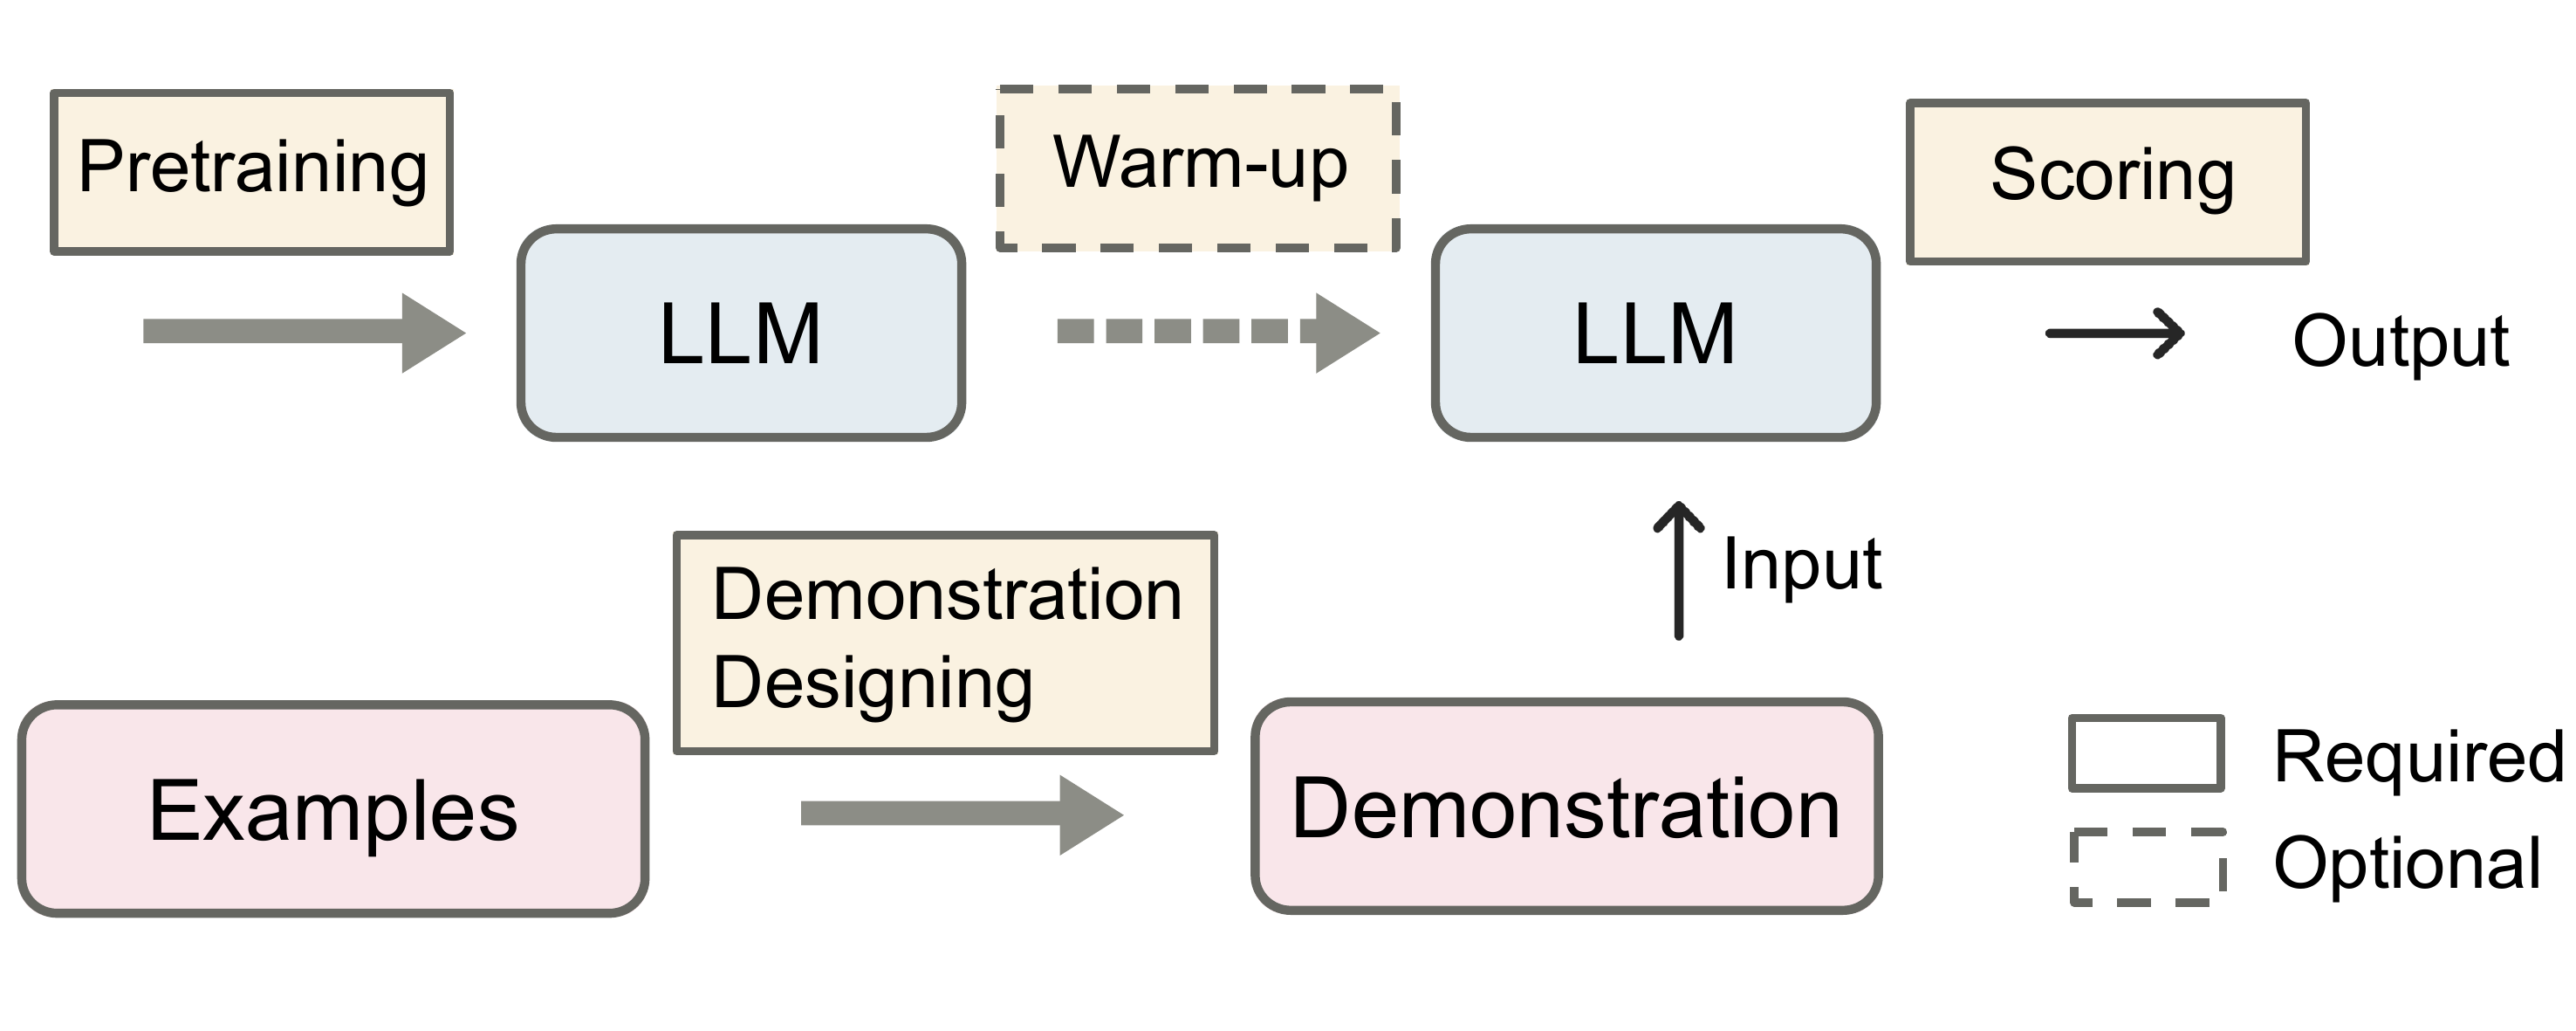}
    \caption{Main procedures of in-context learning.}
    \label{fig:icl_process}
\end{figure}

% \section{Comparison with Finetuning}
% \begin{figure}[t!]
%     \centering
%     \includegraphics[width=0.9\linewidth]{fig/icl_ft.pdf}
%     \caption{Main procedures of in-context learning.}
%     \label{fig:icl_ft}
% \end{figure}
