# Supplementary material for: A Survey on In-context Learning
Source: arXiv:2301.00234 source file (2024-10-05)
Supplement: Supplementary file 2 [file multimodal_sim.tex]

% Multimodal Applications
% Due to the great success of ICL in the area of NLP, the idea also has motivated pilot studies toward investigating the ICL ability in visual and multimodal tasks.
The tremendous success of ICL in NLP  has inspired researchers to explore its potential in different modalities. In the visual field, ICL capabilities for tasks like image segmentation and image generation are robustly demonstrated\cite{bar2022visual_icl,wang2023imagesPainter,wang2023seggpt,wang2023prompt_diffusion}. Retrieval technique\citet{zhang2023visual_icl_analysis} and prompt fusion technique\citet{sun2023exploring_visual_icl} are examined to enhance outcomes.
% \subsection{Multi-Modal In-Context Learning}
In the vision-language domain, a vision encoder paired with a frozen language model demonstrates multi-modal few-shot learning capabilities after training\citep{tsimpoukelli2021frozen, alayrac2022flamingo}.
Kosmos-1\citep{huang2023kosmos},METALM\citep{hao2022language},ICL-D3IE\citep{he2023icld3ie},Recent advancements include creating instruction tuning datasets from existing vision-language tasks or with advanced LLMs like GPT-4, connecting LLMs with powerful vision foundational models like BLIP-2 for multi-modal learning\citep{xu2022multiinstruct,li2023otter,liu2023llava,zhu2023minigpt4,dai2023instructblip}.
 % integrates a vision encoder with LLMs for enhanced ICL across multi-modal tasks\citep{alayrac2022flamingo}. 
 % Similarly, Kosmos-1 exhibits zero-shot, few-shot, and multi-modal chain-of-thought prompting abilities \citep{huang2023kosmos}. METALM introduces a semi-causal language modeling objective to achieve strong ICL performance across vision-language tasks \citep{hao2022language}. The ICL-D3IE approach employs a novel ICL framework that iteratively updates diverse demonstrations—including hard, layout-aware, and formatting demonstrations to train LLMs for enhanced document information extraction (DIE)\citep{he2023icld3ie}. 
% \subsection{Speech In-Context Learning}
In the speech area, ~\citet{wang2023neural} treated text-to-speech synthesis as a language modeling task and and propose the first TTS framework with strong ICL capability. Subsequently, VALLE-X~\citep{zhang2023valle-x} extend the idea to zero-shot cross-lingual text-to-speech synthesis and zero-shot speech-to-speech translation tasks.
