# Supplementary material for: A Survey on In-context Learning
Source: arXiv:2301.00234 source file (2024-10-05)
Supplement: Supplementary file 3 [file related_concept.tex]

\paragraph{Few-shot Learning}

\paragraph{Fine-tuning}

\paragraph{Prompt Predicting}

\paragraph{Instruction Tuning}
